# Supplementary material for: Omnigrasp: Grasping Diverse Objects with Simulated Humanoids
Source: arXiv:2407.11385 source file (2025-05-18)
Supplement: Supplementary file 1 [file supp_divserse.tex]

\begin{figure}
\begin{center}
\includegraphics[width=\textwidth]{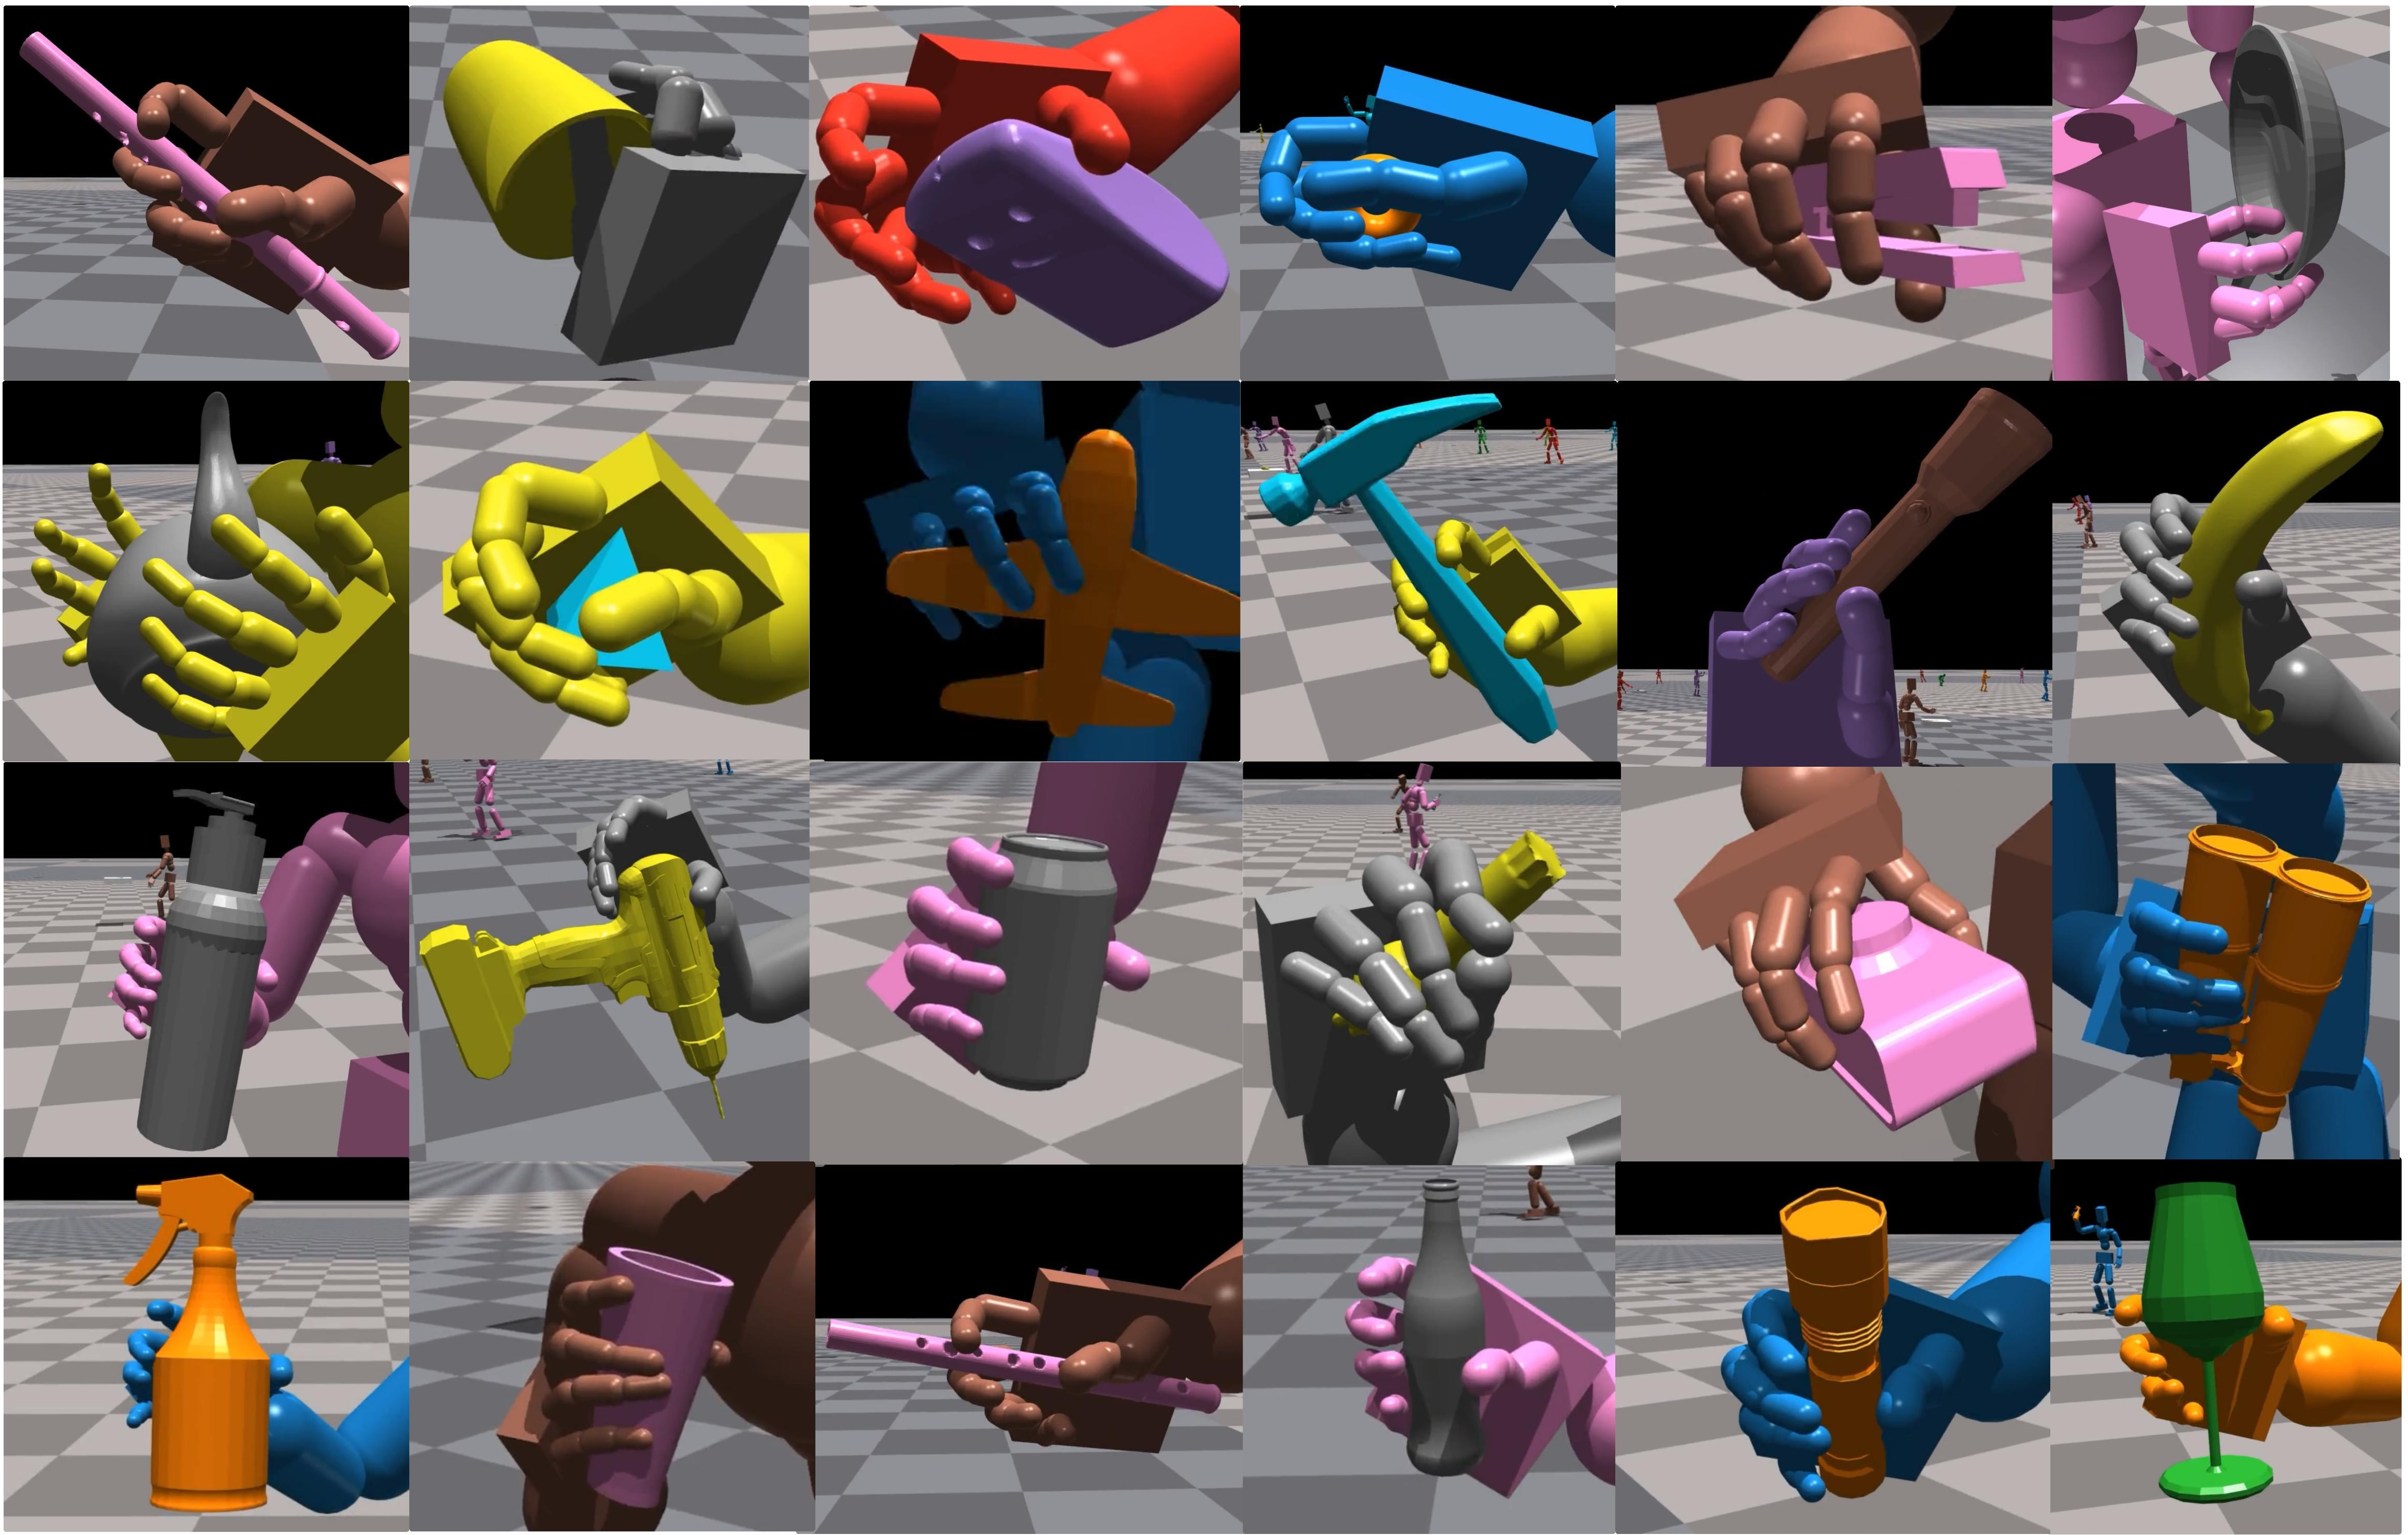}
\end{center}
   \caption{\small   $\name$  uses diverse strategies to grasp objects of different shapes. }
\label{fig:supp_diverse}

\end{figure}
